# Supplementary material for: FLAASH: Flexible Accelerator Architecture for Sparse High-Order Tensor Contraction
Source: arXiv:2404.16317 source file (2024-04-25)
Supplement: Supplementary file 1 [file 6_appendix.tex]

\begin{table}[h]
    \caption{Versions of software packages.}%
    \label{tab:versions}
    \centering
    \begin{tabular}{lc}
        \toprule
        Software & Version \\
        \midrule
        SystemC  & 2.3.2-2 \\
        g++      & 12.2.1  \\
        Make     & 4.4.1   \\
        \midrule
        Python   & 3.10.10 \\
        Sparse   & 0.14.0  \\
        Linux    & 6.1.25  \\
        \bottomrule
    \end{tabular}
\end{table}

Anything besides this table?
I could also include any other plots, but I'm not sure what else needs plotting.
